# Supplementary material for: Traffic disruption modelling with mode shift in multi-modal networks
Source: arXiv:2210.06115 source file (2022-10-12)
Supplement: Supplementary file 1 [file appendix.tex]

\clearpage

  \appendix 

This document is accompanying the submission \textit{\titlename}.
The information in this document complements the submission, and it is presented here for completeness reasons. It is not required for understanding the main paper, nor for reproducing the results.

This section aims to extend the concept and provide more details of the integrated OD estimation methodology for multiple transport modes. As described in (\textit{Stage 2}) of \cref{Fig_research_framework}, the traditional OD estimation belongs to the trip distribution step (\textit{Step 2}) of the static demand estimation, where the input source for this step is the vectors of trip generation and attraction, aggregated by mean of transports. These vectors only indicate the total number of production and attraction for each pre-defined zones. The directed trip matrix \textit{Output 2)} is then produced at \textit{Step 2}, also aggregated by the mean of transports. In the following \textit{Step 3}, the \textit{Output 2} is used as the cost matrix in a modal split utility function for estimating the travel utility for each OD pair and each transport mode. Based on the travel utility, the probability of mode choice is obtained from a modal split discrete choice function, where the transport-mode-disaggregated travel matrix is generated for the Trip assignment step (\textit{Step 5}). 

The above section briefly introduces the traditional procedures for OD estimation that are established on \textit{Trip generation and attraction (Step 1)} estimated by using a multinomial regression function with parameters captured from Census or survey data. However, since the availability of big traffic data (e.g. traffic count data or mean road section-based travel speed data) and transport usage data (e.g. public transport tap-on and tap-off data), the estimation method for travel demand is changed accordingly to a data-driven-oriented method, that is capable of producing a higher-quality and more accurate travel demand. The following section introduces the method of utilising the traffic and transport usage data when demand estimating for car and public transport networks. 

\subsection{Methodology of integrated OD estimation by gravity model}
\subsubsection{Nomenclature}
\begin{table}[H]
\caption{Nomenclature}
\centering
\begin{tabular}{l|l}
    \hline \hline
    Notation & Definition\\ 
    \hline
    \multicolumn{2}{l}{Parameters} \\
    \hline
    $i$ & Origin zone at which the trip is departing, $i=1...J$ \\
    $j$ & Destination zone at which the trip is arriving, $j=1...J$ \\
    $Z_j$ & Statistical area covered in the study network, $j=1...J$ \\
    $J$ & The total number of statistical areas inside the sub-network\\
    $k$ & Transit modes, consisting of vehicle groups \\
    & and public transport groups \\
    $v$ & Vehicle group, consisting of cars and trucks \\    
    $OD_k$ & OD matrix of vehicle group movements \\
    $OD_c$ & OD matrix of car movements \\    
    $OD_{tk}$ & OD matrix of truck movements \\
    $pt$ & The public transport group, consisting of buses and trains \\
    $OD_{pt}$ & OD matrix of public transport group movements \\
    $OD_b$ & OD matrix of buses \\
    $OD_{tn}$ & OD matrix of trains \\
    \hline
    $T_{i,j}^k$ & Number of trips departing from \\
    & zone $i$ and arriving at zone $j$ by transit mode $k$\\
    $o_{i}^k$ & The total number of trips departing \\
    & from zone $i$ by transit mode $k$ \\
    $A_{i}^k$ & Time-dependent weights against the \\
    & total number of trips departing from an \\
    & origin zone $(o_{i}^k)$ \\
    $d_{j}^k$ & The total number of trips arriving at \\
    & zone $j$ by transit mode $k$ \\
    $B_{j}^k$ & Time-dependent weights against the \\
    &total number of trips arriving at a destination $(d_{j}^k)$ \\
    $P_{i}^k$ & Probability of passenger choosing to \\
    & travel from an origin zone $i$ by transport mode $k$ \\
    $P_{j}^k$ & Probability of passenger choosing to travel to \\
    & a destination $j$ by transport mode $k$ \\
    $c_{i,j}^k$ & Travel cost between a pair of OD by transport mode $k$ \\  
    $\alpha$ & Power of the travel cost \\
    $\beta$ & Exponential weight of the travel cost \\

    $c_{i,j}^{id,k}$ & Intersection delay\\
    
    $c_{i,j}^{sd,k}$ & Section delay\\   
    
    $c_{i,j}^{tp,k}$ & Turn penalty\\

    $s$ & The $s^{th}$ travel cost parameter, $s=1\dots S$ \\
    $z$ & The $z^{th}$ travel cost parameter of \\
    & public transport, $z=1\dots Z$ \\
    $\gamma$ & The $z^{th}$ The weight factor by cost parameter and $X$ \\ 
    $X$ & The cost parameters \\

    $r$ & Count of an iterative calculation \\
    $r_{max}$ & Pre-defined maximum count of an iterative calculation \\
    
    \hline
    $T_{m_i,n_j}^{pt}$ & Number of time-dependent trips departing from \\
    & origin public transport stop $m$ at origin zone $i$, \\
    & and arriving at the destination stop $n$ at zone $j$ \\
    
    $C_{m_i}^{pt}$ & The capacity of an origin public transport stop $m$ \\
    $C_{n_j}^{pt}$ & The capacity of a destination public transport stop $n$ \\

    $t_{m_i,n_j}^{iv,pt}$ & In-vehicle travel time by public transport \\
    $t_{m_i,n_j}^{w,pt}$ & Waiting time by public transport \\    
    $t_{m_i,n_j}^{wa,pt}$ & Walking time, consisting of \\
    & access and egress walking time and \\
    & in-station walking time\\
    $t_{m_i,n_j}^{td,pt}$ & Transfer delay at a public transport stop \\      
    $c_{m_i,n_j}^{f,pt}$ & Fare cost by public transport \\ 
    $c_{m_i,n_j}^{df,pt}$ & Discomfort factor when travelling by public transport \\ 
    
    $P_{m_i}^{pt}$ & Probability of passenger choosing to \\
    & travel from a origin stop $m$ at \\
    & zone $i$ by public transport \\  
    $P_{n_j}^{pt}$ & Probability of passenger choosing to \\
    & travel to a destination stop $n$ at \\
    & zone $j$ by public transport \\
    \hline \hline
\end{tabular}
\end{table}

\subsubsection{Gravity model for OD estimation}
This section aims to extend the concept and provide more details of the integrated OD estimation methodology for multiple transport modes. The OD estimation belong to the trip distribution step (\textit{Step 2}) of a static demand estimation (\textit{Stage 2}) in \cref{Fig_research_framework}. 

Following the zone definition in \cref{II_B_Integrated_OD_estimation}, the vehicle group, $v$, is composed of cars and trucks, where the unit of its OD matrix is defined as the number of vehicles, and the content of the OD matrix are the total number of trips during a time interval $t$. In this study, the interval time $t$ is defined as 15 minus according to the available real data sets.:
\begin{itemize}
\item ${OD}_c(t)=\left[{T}_{i,j}^c(t)\right],\ i,j=1\ldots J$, where ${T}_{i,j}^c$ stands for the number of car trips originating from zone $i$ and arriving at zone $j$ at time interval $t$. 
\item ${OD}_{tk}(t)=\left[{T}_{i,j}^{tk}(t)\right],\ i,j=1\ldots J$, where ${T}_{i,j}^{tk}$ stands for the number of truck trips originating from zone $i$ and arriving at $j$ at time interval $t$. 
\end{itemize}

The public transport group, $pt$, is composed of the movements of buses and trains, where the unit of its OD matrix is defined as the number of passengers, and the content of the OD matrix is the total number of passenger trips:
\begin{itemize}
\item ${OD}_b(t)=\left[{T}_{i,j}^b(t)\right],\ i,j=1\ldots J$, where ${T}_{i,j}^b$ stands for the number of bus trips originating from zone $i$ and arriving at zone $j$ at time interval $t$. 
\item ${OD}_{tn}(t)=\left[{T}_{i,j}^{tn}(t)\right],\ i,j=1\ldots J$, where ${T}_{i,j}^{tn}$ stands for the number of train trips originating from zone $i$ and arriving at zone $j$ at time interval $t$. 
\end{itemize}

The existence of trips between each OD pair depends on the available path for vehicles:
\begin{itemize}
\item if there is no available path between zone $i$ and zone $j$ via mode $k$, then, the number of trips by mode $k$ is zero, therefore, the matrix of trips is an empty matrix: ${T}_{i,j}^k=0$;

\item otherwise, we propose the following methods for a multi-modal OD estimation:
\end{itemize}

    \paragraph{Gravity model for transport OD estimation by a zone-to-zone approach}
    
    \textbf{The gravity model:}
    The number of time-dependent trips by mode k departing from zone $i$ to zone $j$ can be calculated by using the Gravity Model \cite{Ortuzar2011} with a given total number of trips departure at zone $i$ by mode $k$, denoted by $o_i^k$, and the number of trips arrivals at zone $j$ by mode $k$, denoted by $d_j^k$: 
    
    \begin{equation} \label{equation 1}
        T_{i,j}^k (t)=A_i^k(t) o_i^k(t) B_j^k(t) d_j^k(t) f(c_{i,j}^k(t)),    
    \end{equation}
    where $A_i^k$ and $B_i^k$ represent the time-dependent weights toward the total number of departures, also known as the trip production ($o_i^k$) and total number of arrivals, also known as the trip attraction ($d_j^k$) separately; $f\left(c_{i,j}^k\right)$ is the deterrence function that represents the time-dependent travel cost between two zones by mode $k$. 
    \\
    \textbf{The constraints:}
    The model is considered to be limited in a close network where the total number of trips departing from a zone $i$ by mode $k$ at time interval $t$ equals the sum of trips that originated from zone $i$ towards each destination zone $j$:
    
    \begin{equation} \label{equation 2}
        o_i^k(t)=\ \sum_{j=1}^{J}{{T}_{i,j}^k(t)}, 
    \end{equation}
    and the total number of trips arriving at a zone $j$ by mode $k$ at time interval $t$ equals the sum of trips that terminated at a zone $j$ from each origin zone $i$:

    \begin{equation} \label{equation 3}
        d_j^k(t)=\ \sum_{i=1}^{J}{{T}_{i,j}^k(t)}
    \end{equation}
    
    The \autoref{equation 2} and \autoref{equation 3} are sets of constraints to the Gravity model (\autoref{equation 1}). Therefore, the time-dependent weights subject to the Gravity model can be transformed from \autoref{equation 1} and \autoref{equation 2} to:

    \begin{equation} \label{equation 4}
        A_i^k(t)=\frac{1}{\sum_{j=1}^{N}{B_j^k(t)}d_j^k(t)f\left(c_{i,j}^k(t)\right)}
    \end{equation}    
    and from \autoref{equation 1} and \autoref{equation 3} to:

    \begin{equation} \label{equation 5}
        B_j^k(t)=\frac{1}{\sum_{i=1}^{N}{A_i^k(t)}o_i^k(t)f\left(c_{i,j}^k(t)\right)}
    \end{equation}    
    \\
    \textbf{The travel behaviour:}
    From this stage, we are able to describe an individual transport mode and route choice in a probability form. The probability of a passenger choosing to depart from zone $i$ by mode $k$ at time interval $t$ equals the total number of trips between zone $i$ and $j$ over the total number of trips arriving at a zone $j$:

    \begin{equation} \label{equation 6}
        P_i^k(t)=\frac{{T}_{i,j}^k(t)}{d_j^k(t)}
    \end{equation}    
    and the probability of a passenger choosing to arrive at a destination j by mode $k$ at time interval $t$ equals the total number of trips between zone $i$ and $j$ divided by the total number of trips departing from a zone $i$: 
   
    \begin{equation} \label{equation 7}
        P_j^k\left(t\right)=\frac{{T}_{i,j}^k\left(t\right)}{o_i^k\left(t\right)}
    \end{equation}
    \\
    \textbf{The deterrence function:}
    The deterrence function $f\left(c_{i,j}^k\right)$ represents the deterrents to travelling between any OD pair. The deterrents are subjective to the travel cost expressed by using the intersection delay $c_{i,j}^{id,k}$, the section delay $c_{i,j}^{sd,k}$ and the turn penalty $c_{i,j}^{tp,k}$, where:
    
    \begin{itemize}
    \item the intersection delay is the function of the intersection volume, the turn conflicted volume, the intersection length and the travel speed inside an intersection
    
    \item the section delay is the function of the section volume, the section capacity, the travel distance and the travel speed on the section
    
    \item the turn penalty is the function of the turn volume or queue at turn, the turn capacity, the turning distance and the turning speed
    \end{itemize}

    Therefore, the integrated travel cost that decreases trips can be denoted as:
    \begin{equation} \label{equation 8}
        c_{i,j}^{integrated,k} = \gamma_0^k + \sum_{s=1}^{S}{\gamma_s^k X_s^k}
    \end{equation}
    where $s=1\dots S$, which indicate the $s^{th}$ different travel cost parameters; $\gamma$ is the weight factor by cost parameter and $X_s$ represents cost parameters, such as the intersection delay $c_{i,j}^{id,k}$, the section delay $c_{i,j}^{sd,k}$ and the turn penalty $c_{i,j}^{tp,k}$. 
    
    The most common and proven practical form of the deterrence function between any two zones $i$ and $j$ is the Gamma function:

    \begin{equation} \label{equation 9}
        f\left(c_{i,j}^k\right)\ ={(c}_{i,j}^k)^\alpha\ e^{-\beta c_{i,j}^k},
    \end{equation}
    where $c_{i,j}^k$ represents the travel cost between a pair of OD by transport mode $k$, $\alpha$ is the power of the travel cost and $\beta$ is the exponential weight of the travel cost. 
    \\

    \textbf{The objective function:}
    The OD estimation based on the Gravity Model is a process of iterative calculation where for each calculation step, the time-dependent weights $(A_i^k)$ and $(B_j^k)$ are updated subjecting to the set of constraints (\autoref{equation 4} and \autoref{equation 5}).The criteria of the convergence are therefore set as the functions:

    \begin{equation} \label{equation 10}
        {cc}^k \geq\max_{i,j}{(\max_i{\left(\frac{A_i^{k,r+1}-A_i^{k,r}}{A_i^{k,r+1}}\right)}, \max_i{\left(\frac{B_j^{k,r+1}-B_j^{k,r}}{B_j^{k,r+1}}\right)} )},
    \end{equation}
    where ${cc}^k$ is the criteria of convergence that defines the acceptable closeness of the last two time-dependent results of the weights, namely $A_i^{k,r+1}$ and $A_i^{k,r}$, and $B_j^{k,r+1}$ and $B_j^{k,r}$, $r$ represents the count of the iterative calculation. Although a higher number of iterative calculations often means a more accurate result, for time and effort saving purposes, the total count of the iterative calculation should also be limited as: 

    \begin{equation} \label{equation 11}
        r\in{1,\ ...,r_{max}},
    \end{equation}
    where $r_{max}$ is the pre-defined maximum number of iterative calculations. 
    
    The above method is used for estimating the zone to zone OD matrix for vehicles in networks following the Gravity model, which requires the travel cost and trip production and attraction by zones. All OD estimation treating the vehicle as the entity, such as private cars and trucks can be estimated following this idea.

    \paragraph{Gravity model for public transport group OD estimation by a stop-to-stop approach}
    
    \textbf{The gravity model:}
    The number of time-dependent trips made by transit mode $k$ is obtained based on the movements of public transport stops. Therefore, the total number of trips departing from an origin stop $m, m=1\dots N$ to a destination stop $n, n=1\dots N$ can be calculated based on the Gravity Model with a given total number of trips departing from the origin stop m by mode $pt$, denoted by $o_{m_i}^{pt}$, and that of trips arriving at a destination stop $n$ by mode $pt$, denoted by $d_{n_j}^{pt}$: 
    
        \begin{equation} \label{equation 12}
            T_{m_i,n_j}^{pt}(t)=A_{m_i}^{pt}(t){o}_{m_i}^{pt}{(t)B}_{n_j}^{pt}{(t)d}_{n_j}^{pt}(t)f\left(c_{m_i,n_j}^{pt}(t)\right),
        \end{equation}
    where $A_{m_i}^{pt}$ and $B_{n_j}^{pt}$ represent the time-dependent weights towards the total number of origins ($o_{m_i}^{pt}$) by public transport and total destinations ($d_{n_j}^{pt}$), separately; $f\left(c_{m_i,n_j}^{pt}\right)$ is the deterrence function that represents the time-dependent travel cost between two zones by mode $pt$, the origin stop $m$ belongs to the origin zone $i$ while the destination stop $n$ belongs to the arrival zone $j$. 
    \\
    \textbf{The constraints:}
    Similarly to the constraints for the vehicular group when using the Gravity Model, the total number of departures by public transport from a public stop $m$ should be equal to the sum of trips that originate from a stop $m$ to each destination stop $n$:
    
        \begin{equation} \label{equation 13}
            o_{m_i}^{pt}(t)=\ \sum_{j=1}^{N}{{T}_{m_i,n_j}^{pt}(t)},
        \end{equation}
    and the total number of trips by public transport arriving at stop $n$ at time interval $t$ equals the sum of trips that terminate at stop $n$ from each origin stop $m$:
    
        \begin{equation} \label{equation 14}
            d_{n_j}^{pt}(t)=\ \sum_{i=1}^{N}{{T}_{m_i,n_j}^{pt}(t)}\ 
        \end{equation}

    The time-dependent weights for the multi-modal public transport movements subject to the Gravity model can now be transformed from \autoref{equation 12} and \autoref{equation 13} to:
    
        \begin{equation} \label{equation 15}
            A_{m_i}^{pt}(t)=\frac{1}{\sum_{j=1}^{N}{B_{n_j}^{pt}(t)}d_{n_j}^{pt}(t)f\left(c_{m_i,n_j}^{pt}(t)\right)}
        \end{equation}
    and from \autoref{equation 12} and \autoref{equation 14} to:
    
        \begin{equation} \label{equation 16}
            B_{n_j}^{pt}(t)=\frac{1}{\sum_{i=1}^{N}{A_{m_i}^{pt}(t)}A_{m_i}^{pt}(t)f\left(c_{m_i,n_j}^{pt}(t)\right)}
        \end{equation}
    \\
    \textbf{The travel behaviour:}
    The probability of a passenger choosing to travel to a destination stop $n$ by public transport at time interval $t$ becomes: 

        \begin{equation} \label{equation 17}
            P_{n_j}^{pt}\left(t\right)=\frac{{T}_{m_i,n_j}^{pt}\left(t\right)}{o_{m_i}^{pt}\left(t\right)}
        \end{equation}    
    and the probability of a passenger choosing to travel from a stop $m$ by public transport at time interval $t$ is obtained by: 
    
        \begin{equation} \label{equation 18}
            P_{m_i}^{pt}(t)=\frac{{T}_{m_i,n_j}^{pt}(t)}{d_{n_j}^{pt}(t)}\ 
        \end{equation}
    \\
    \textbf{The deterrence function:}    
    The deterrence function $f\left(c_{m_i,n_j}^{pt}\right)$ that represents the disincentives of travelling between an OD pair has different elements comparing to that of a vehicular group. The disincentives parameters of the public transport travel cost include: origin and destination stops ($c_{m_i}^{pt}$ and $c_{n_j}^{pt}$), in-vehicle travel time($t_{m_i,n_j}^{iv,pt}$), waiting time($t_{m_i,n_j}^{w,pt}$), walking time ($t_{m_i,n_j}^{wa,pt}$), transfer delay ($t_{m_i,n_j}^{td,pt}$), fare cost ($c_{m_i,n_j}^{f,pt}$) and discomfort factor($c_{m_i,n_j}^{df,pt}$).

    Therefore, the integrated travel cost that decreases trips of the public transport users can be described as:
    \begin{equation} \label{equation 19}
        c_{i,j}^{integrated,pt} = \gamma_0^{pt} + \sum_{z=1}^{Z}{\gamma_z^{pt} X_z^{pt}}
    \end{equation}
    where $s=1\dots S$, which indicate the $s^{th}$ different travel cost parameters; $\epsilon$ is the weight factor by cost parameter and $X_s$ represents cost parameters, such as those mentioned above.

    The form of the deterrence function that can be used here is the Gamma function:
        \begin{equation} \label{equation 20}
            f\left(c_{m_i,n_j}^{pt}\right)\ ={(c}_{m_i,n_j}^{pt})^\alpha\ e^{-\beta c_{m_i,n_j}^{pt}}
        \end{equation}

    The criterion of the convergence follows either \autoref{equation 11} or the functions that similar to \autoref{equation 10}: 

        \begin{equation} \label{equation 21}
            {cc}^{pt}\ \geq\max_{i,j}{(\max_i{\left(\frac{A_{m,i}^{pt,r+1}-A_{m,i}^{pt,r}}{A_{m,i}^{pt,r+1}}\right)},\ \max_i{\left(\frac{B_{n,j}^{pt,r+1}-B_{n,j}^{pt,r}}{B_{n,j}^{pt,r+1}}\right)}\ )}
        \end{equation}
    where ${cc}^{pt}$ is the criteria of convergence that defines the acceptable closeness of last two time-dependent weights, $r$ is the count of iterative calculations. The criteria for breaking the iterative calculation follows \cref{equation 11}.
